# Supplementary material for: Narrow-line single-molecule transducer between electronic circuits and surface plasmons
Source: arXiv:1509.03987 source file (2015-09-14)
Supplement: Supplementary file 1 [file SupplementaryInformation.pdf]

# Narrow-line single-molecule transducer between electronic circuits and surface plasmons.

Michael C. Chong, Gaël Reecht, Hervé Bulou, Alex Boeglin, Fabrice Scheurer, Fabrice Mathevet, Guillaume Schull

## CONTENTS

S1 – Detailed study of the on-surface polymerization products. 2

S2 – Experimental procedure used to lift a molecular wire in the STM junction. 4

S3 – TD-DFT simulations of the excited and ground states. 5

S4 – DFT simulations of the Raman spectra 6

S5 – Vibronic spectra of different emitters. 8

S6 – Experimental determination of $\gamma_{exc}$ vs $E(r, h\nu)$. 10

References 12

**S1 – Detailed study of the on-surface polymerization products.**

Figure S1a shows a large scale STM image of a Au(111) surface after co-deposition of 5,5”-dibromo-2,2’:5’,2”-terthiophene and 5,15-(diphenyl)-10,20-(dibromo)porphyrin (Fig. 1a of the main manuscript) and subsequent heating of the surface at ≈ 580K. This image reveals several copolymers of different sizes and compositions as well as individual molecules whose shape is reminiscent of the porphyrin. In the enlarged STM image in Fig. S1b a symmetric (I) and an antisymmetric (II) conformation of the isolated molecules can be distinguished. A close inspection of the molecule within the molecular chain reveals the same two conformations.

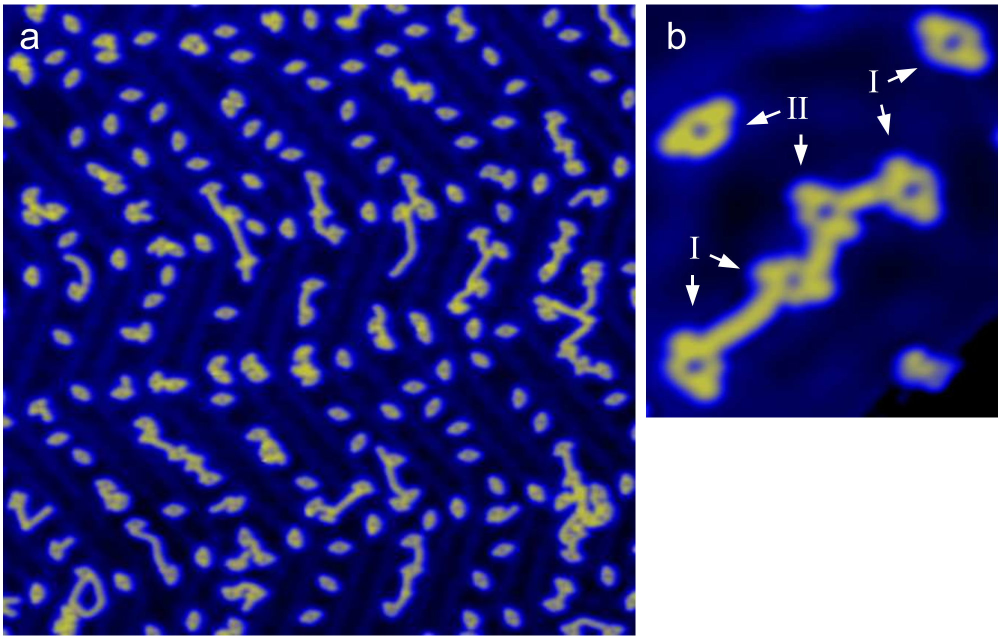


FIG. S1. (a) Large scale STM image ($57 \times 57$ nm$^2$, $I = 0.1$ nA, $V = 0.1$ V) after the on-surface polymerization of 5,5”-dibromo-2,2’:5’,2”-terthiophene and 5,15-(diphenyl)-10,20-(dibromo)porphyrin on Au(111). (b) Enlarged STM image ($8.6 \times 10$ nm$^2$, $I = 0.1$ nA, $V =$ -0.1 V) revealing the presence of symmetric (I) and antisymmetric (II) molecular species.

To determine the chemical nature of these molecules we deposited 5,15-(diphenyl)porphyrin (H2-DPP) molecules on a Au(111) kept at 4.5K. The STM image in Fig. S2a reveals two bright lobes at the extremities of the molecule. These lobes correspond to the lateral phenyl rings of H2-DPP that are tilted with respect to the core of the molecule (Fig. S2c) which

explains their brighter contrast in the STM images. Only one conformer is observed in this case. The sample was then heated at ≈ 580K. On the STM images recorded after this procedure (e.g., Fig. S2b), the phenyl rings have now the same intensity, suggesting that they are co-planar with the porphyrin core. This is only possible if cyclodehydrogenation reactions occur, resulting in configurations where the benzene rings are fused to the porphyrin core (Fig. S2d). Here, a symmetric and an antisymmetric conformations are distinguished as observed in Fig. S1. These conformations respectively correspond to cases where the two cyclodehydrogenations reactions occurred on the opposite (I) and on the same side (II) of the porphyrin core. Similar cyclodehydrogenation reactions were reported recently[1] for tetraphenylporphyrin molecules deposited on Ag(111). Suspended copolymers containing symmetric and antisymmetric fused-H2P present indiscernible optical spectra.

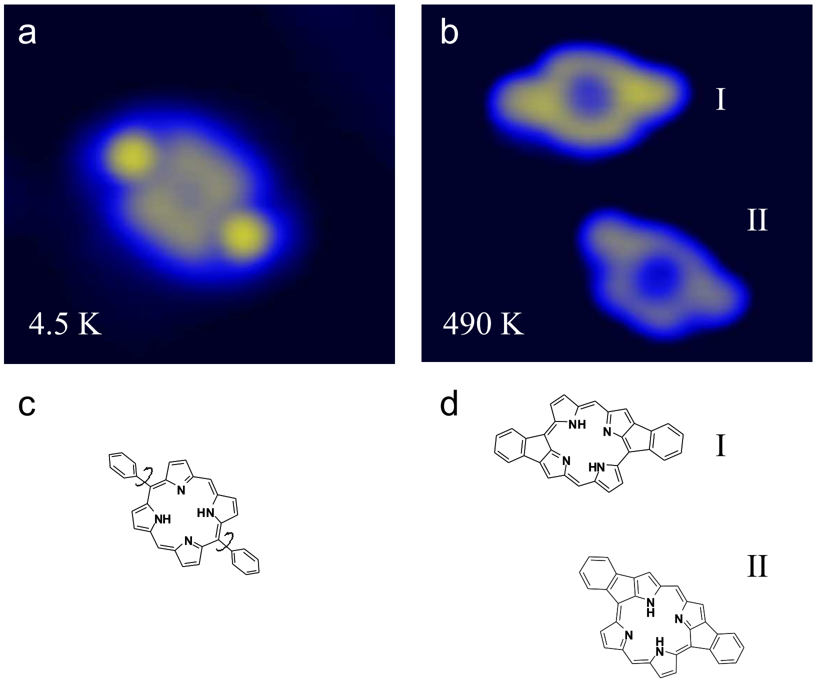


FIG. S2. (a) STM image of a 5,15-(diphenyl)porphyrin (3.7 × 3.4 $nm^2$, $I$ = 0.1 nA, $V$ = -1.5 V) deposited on a cold (4.5 K) Au(111) sample. (b) STM image of the same sample (3.7 × 3.4 $nm^2$, $I$ = 0.03 nA, $V$ = -0.3 V) after heating at ≈ 580K. (c) and (d) Models of the observed molecular species.

**S2 – Experimental procedure used to lift a molecular wire in the STM junction.**

As a first step, the tip of the STM is located on top of the extremity of the targeted wire. In all reported cases the wires are terminated by a fused-H2P molecule. The STM tip is then approached to the center of the fused-H2P up to the formation of a contact between the tip and the molecule. Figure S3 shows a conductance curve (black line) recorded during this procedure. The point of contact (dashed arrow), which appears as an inflexion in the conductance curve, defines the origin of the abscissa. The conductance curve recorded during the retraction of the tip appears as a blue line in Fig. S3. The slope of this curve is milder than the one recorded during the approach, attesting the presence of the molecular wire in the junction[2,3].

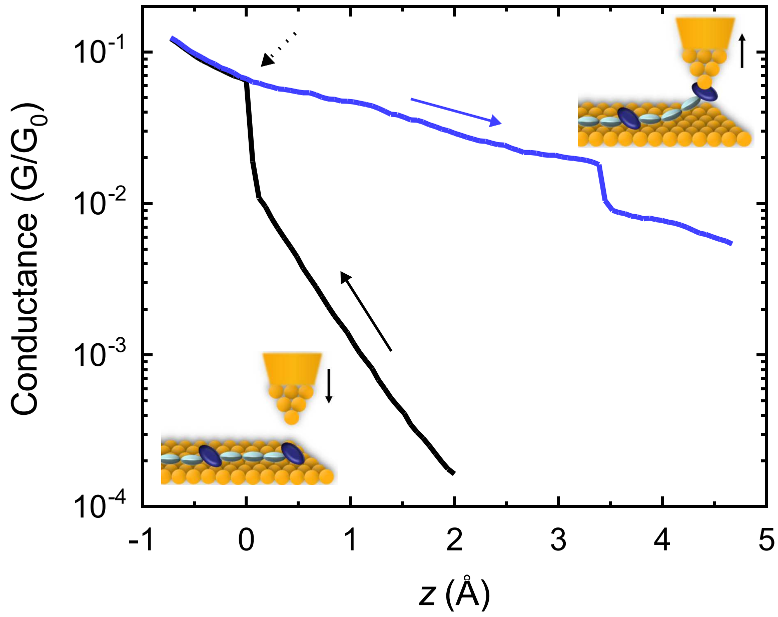


FIG. S3. Conductance curves ($V$ = -0.1 V) recorded during the approach (black curve) and the retraction (blue curve) of the STM tip to the center of a fused-H2P located at the extremity of a molecular wire. The dashed arrow indicates the point of contact. Sketches of the procedures appear in inset.

**S3 – TD-DFT simulations of the excited and ground states.**

Electronic structure calculations have been performed with the Gaussian 09 (Revision B.01) software[4] using the DFT approach at the PBE (Perdew, Burke and Ernzerhof 1996 exchange and gradient corrected correlation functionals) and Becke's 1993 (three parameter hybrid functional) B3LYP/6-31G(d,p) level of accuracies to optimize the geometrical structures of unsubstituted or mono- or di-terThiophene substituted diphenylporphyrins (H2-DPP) or its fused isomers (fused-H2P) in the symmetric conformation. Excited singlet states have then been calculated through the TD-DFT methodology at the B3LYP/6-31G(d,p) level of theory. Since only the lowest two transitions were of interest, only 16 converged roots were asked for. No significant differences have been recognized between results obtained from BPE vs. B3LYP geometries.

Our calculations (Table 1) concerning the optical gaps agree with the experimental emission energy provided that the chromophore is the fused-H2P. Indeed, the optical gap values for all the H2-DPP derivatives are far too large. These results also show that the terthiophene chains have a minor impact (0.025 eV) on the So→S1 transition energy of the fused-H2P.

TABLE I. Singlet excitation energies in eV

| Transition | H2-DPP | terT-H2-DPP | diterT-H2-DPP | fused-H2P | terT-fused-H2P | diterT-fused-H2P |
|---|---|---|---|---|---|---|
| $S_0 \to S_1$ | 2.1694 | 2.1514 | 2.0647 | 1.5076 | 1.4962 | 1.4826 |
| $S_0 \to S_2$ | 2.3130 | 2.2791 | 2.1843 | 1.8688 | 1.7912 | 1.7397 |

In the above table, the fused-H2P structure has both central H atoms on the pyrrole rings, the most stable isomer according to the total energies of the system at the optimum geometry. The alternate configuration having the H's on the nitrogens of the fused rings has been found less stable by 0.1820 eV and leads to singlet transition energies of 1.6260 eV to $S_1$ and of 1.9840 eV to $S_2$. Finally, the mixed situation where both H atoms are in cis produced the two lowest transitions at 1.5436 eV and at 1.9013 eV, more in line with the most stable structure but at the cost of a total ground state energy destabilization of 0.6362 eV. Nevertheless, since the H atoms may tunnel from one nitrogen to the next treating their nuclei as classical fixed particles may be a source of error.

## S4 – DFT simulations of the Raman spectra

The relatively uniform intensities of the weak features detected in the experimental luminescence spectra and the non-linearity in their progression suggest that they may involve 0-1 vibronic transitions of the emitter. Furthermore, since the strong peak observed in luminescence corresponds to the S0→S1 transition of the fused-H2P, the vibronic features should belong to modes that are optically active in a transition of strong $\pi$ to $\pi^*$ character, namely in-plane and symmetric (Raman-active) modes. The analysis of the normal modes and of their Raman activities for the fused-H2P and H2-DPP molecules turns out to provide further evidence pointing to the actual structure of the light emitting unit (Fig. S4). The computations have been performed (more details are given in the previous S3 Section) using the PBE exchange and correlation functionals with the 6-31G(d,p) basis set.

The proposed structure for fused-H2P has C2h symmetry and since IR-active and out-of-plane modes are irrelevant in a first analysis, only the Raman activities of the modes belonging to the $A_g$ representation have been used in the simulation of the Raman spectrum of fused-H2P. The qualitative similarity between the features of the computed Raman spectrum (Fig. S4b) and of the luminescence (Fig. S4a) is quite convincing in the fingerprint region from 800 cm$^{-1}$ to 1700 cm$^{-1}$. At lower frequencies, the agreement is elusive as both the activities and distribution of the modes do not compare favorably. This may however be explained through the binding of the fused-H2P to terthiophene units and to their connection to the STM tip and Au surface. Consideration of $B_g$ modes and inclusion of terthiophene units in the DFT calculations have not conclusively improved the identification of the vibronic features.

The vibrational modes of H2-DPP have been computed for the geometry presenting the C2 symmetry (Fig. S4c). The distribution of the modes through the fingerprint region as well as their Raman activities are quite different from those computed for fused-H2P. The analysis shows that this is due to the presence of four Pyrrole rings (whereas only two remain in the fused structure) and to the deformation modes of the Phenyl substituents (absent in fused-H2P). Together with the transition energy calculations presented in the previous Section, these findings indicate that the initialy deposited bromated H2-DPP has indeed undergone fusion of the phenyls.

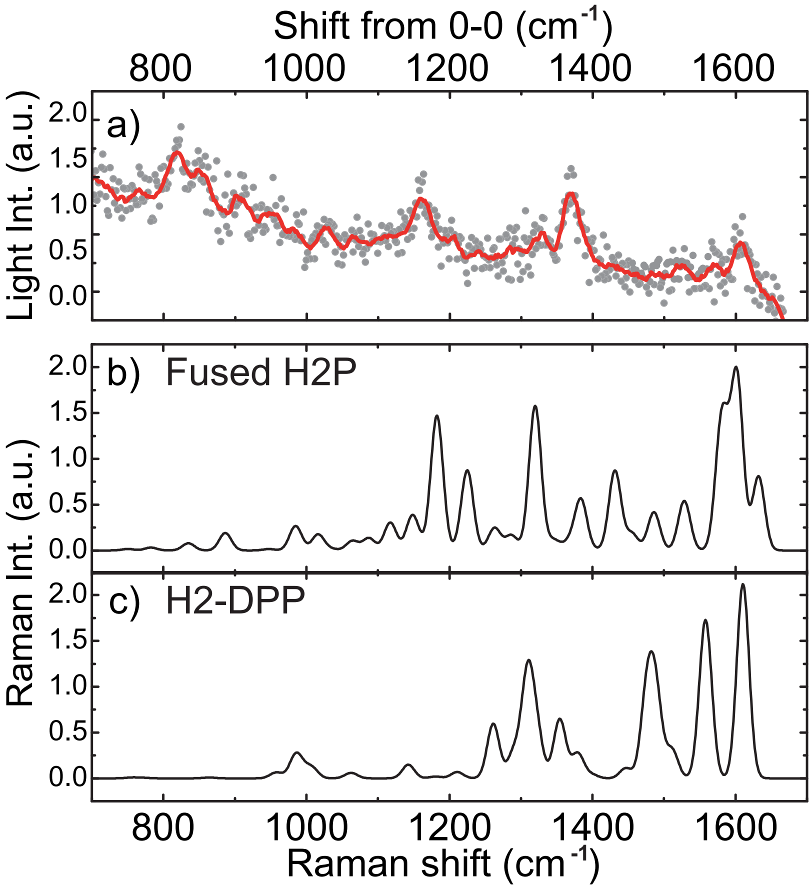


FIG. S4. (a) Experimental vibronic spectra of figure 3b compared to the calculated Raman spectra of (b) fused-H2P and (c) H2-DPP. The spectra is limited to the high frequency region (800 to 1700 cm$^{-1}$) where the identification of vibrational modes is reliable.

**S5 – Vibronic spectra of different emitters.**

Figure S5 displays experimental vibronic spectra of different emitters (acquired with low (a, b, c) and high (d, e) spectral resolutions) compared to the calculated Raman spectra of fused-H2P (f). This figure shows that the modes appear at essentially the same energy from emitter to emitter, but that the relative intensity of the modes may vary. This is likely due to variations of the structural (*e.g.,* thiophene chains, atomic structure of the tip or sample...) and electromagnetic (*i.e.,* the surface plasmons) environment.

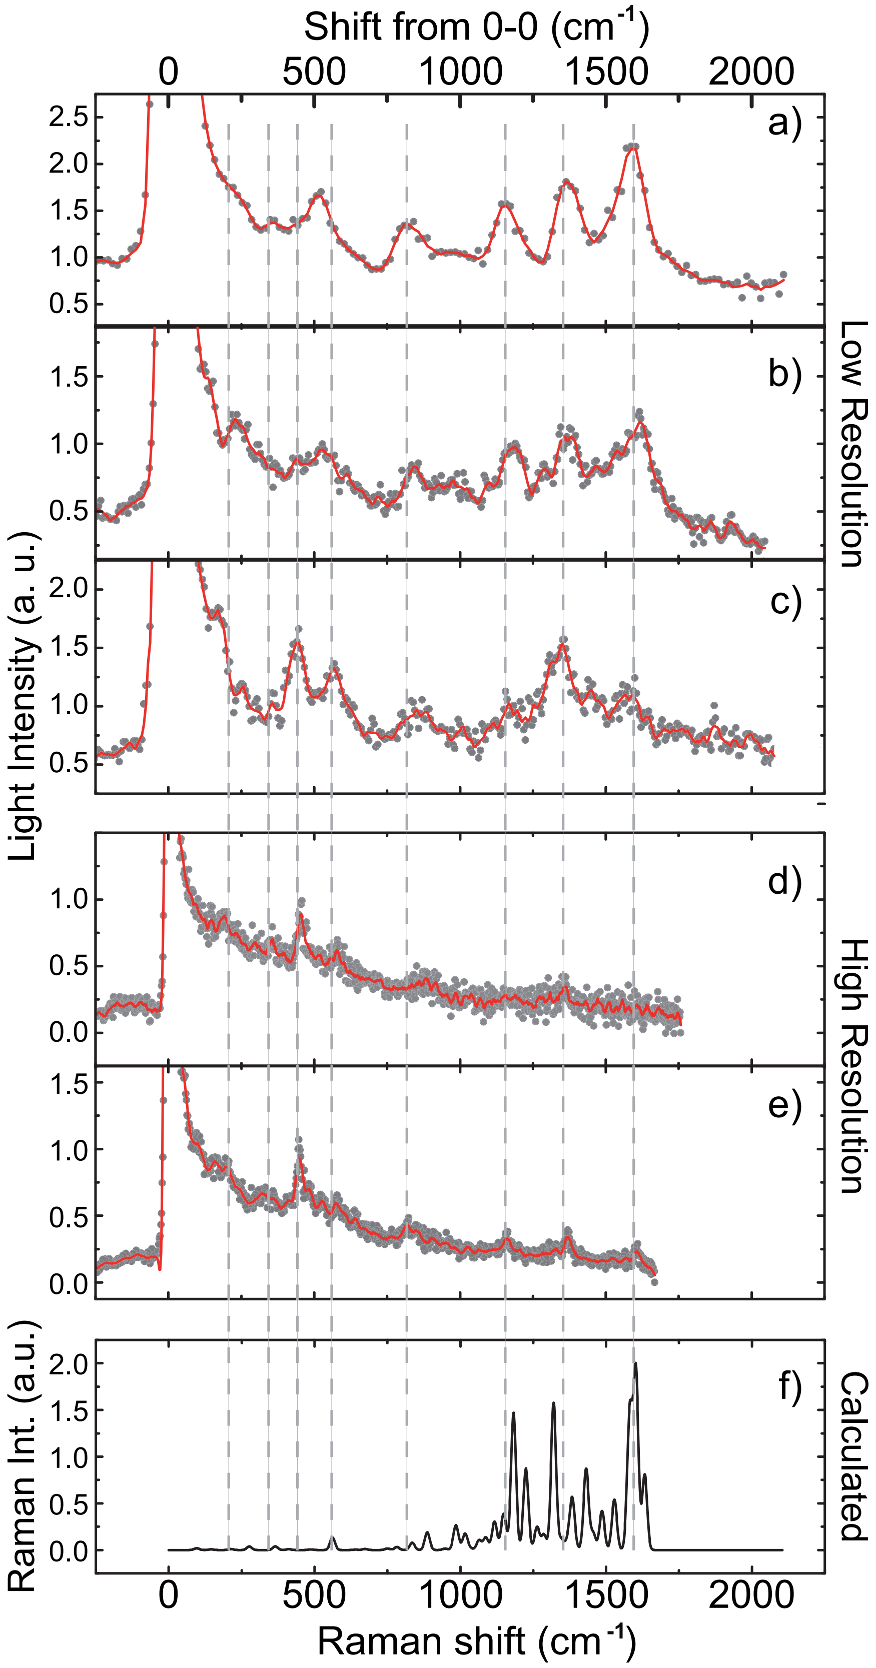


FIG. S5. (a) Experimental vibronic spectra of different emitters acquired with low (a, b, c) and high (d, e) spectral resolutions compared to the calculated Raman spectra of fused-H2P (f).

## S6 – Experimental determination of $\gamma_{exc}$ vs $E(r, h\nu)$.

The fluorescence rate of a single molecular emitter close to a laser irradiated gold nanostructures follows:

$$\gamma_{em} = \gamma_{exc}\, Q, \tag{1}$$

Where $\gamma_{exc}$ is the emitter excitation rate and $Q$ its photon emission probability[5]. Here, $\gamma_{exc} \propto E^2(z, h\nu)$ where $E(z, h\nu)$ is the local electromagnetic field intensity at the molecule position $z$ and at the molecule fluorescence energy $h\nu$. In such an experiment, $E^2(z, h\nu)$ directly scales with the laser intensity and a plasmon amplification function related to the nanoparticule.

Based on the optical spectra in Fig. 4a, we assumed a similar emission mechanism in our experiment, at the exception that the plasmons are originally excited by inelastic tunnelling electrons crossing the STM junction. Assuming a constant density of electrode states, we can write:

$$E^2(z, h\nu, V) \propto I\, \Gamma(h\nu)(eV - h\nu) \tag{2}$$

Where $I$ is the tunnelling current intensity, $\Gamma(h\nu)$ is the electromagnetic density of states of the pristine tip-surface junction and where $(eV - h\nu)$ accounts for the impact of the bias voltage. $\Gamma(h\nu)$ is affected by the chemical nature and the nanoscopic shape of the electrodes[6], and is determined experimentally by recording an optical spectra with the pristine junction[3]. Knowing the intensity $I$ of the tunnelling current and the plasmon amplification function $\Gamma(h\nu)$, it is therefore possible to estimate the voltage dependency of the local electromagnetic field $E(z, h\nu, V)$ felt by the emitter. Figure S6a displays 3 optical spectra of Fig. 4a (the spectra recorded at 1.54 V was not considered because the light intensity was too low) together with the associated $E^2(z, h\nu, V)$ spectra. In Fig. S6 (and inset of Fig. 4a in the manuscript) we visualize the variation of the number of emitted photons per second, $\gamma_{em}$, integrated over a 20 meV window around the 0-0 transition ($h\nu = 1.54$ eV) as a function of the electromagnetic field intensity variations averaged over the same energy window. This plot reveals that $\gamma_{em} \propto E^2(z, h\nu, V)$. Note that the emission probability $Q$ is also impacted by the electromagnetic density of states $\Gamma(h\nu)$. However, $\Gamma(h\nu)$ is the same for these 3 spectra, implying that $Q$ is constant and $\gamma_{em}$ only depends on $\gamma_{exc}$.

We can therefore show that $\gamma_{exc} \propto E^2(z, h\nu, V)$ in our experiment. This observation confirms the plasmonic excitation of the molecular emitter, a behaviour that was never reported for

a single-molecule in a STM junction.

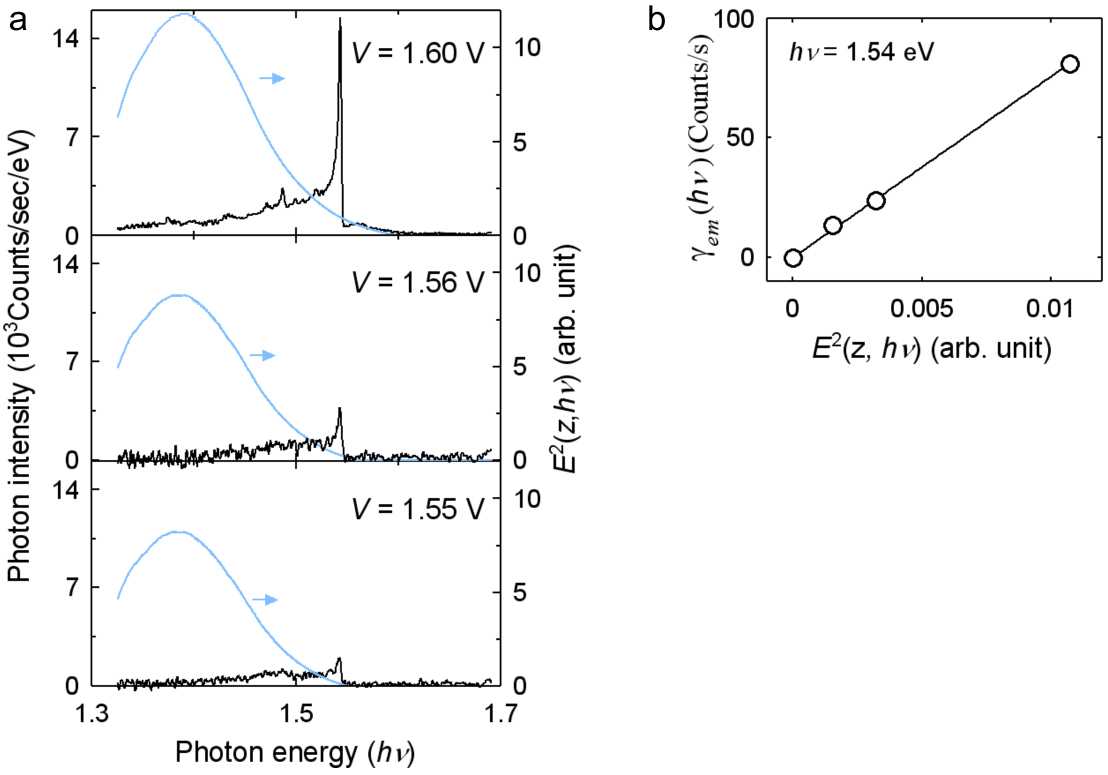


FIG. S6. (a) Light spectra (black lines) of a suspended copolymer as a function of voltage ($z =$ 2.1 nm, high resolution grating) and associated squared local electromagnetic field $E^2(z, h\nu, V)$ felt by the emitter (blue lines). (b) Emission rate as a function of $E^2(z, h\nu)$ integrated over a 20 meV energy window around the 0-0 peak for the spectra in (a).

[1] A. Wiengarten, J. A. Lloyd, K. Seufert, J. Reichert, W. Auwärter, R. Han, D. A. Duncan, F. Allegretti, S. Fischer, S. C. Oh, O. Saglam, L. Jiang, S. Vijayaraghavan, D. Écija, A. C. Papageorgiou, and J. V. Barth, Chem. Eur. J. **21**, 12285 (2015).

[2] L. Lafferentz, F. Ample, H. Yu, S. Hecht, C. Joachim, and L. Grill, Science **323**, 1193 (2009).

[3] G. Reecht, F. Scheurer, V. Speisser, Y. J. Dappe, F. Mathevet, and G. Schull, Phys. Rev. Lett. **112**, 047403 (2014).

[4] M. J. Frisch, G. W. Trucks, H. B. Schlegel, G. E. Scuseria, M. A. Robb, J. R. Cheeseman, G. Scalmani, V. Barone, B. Mennucci, G. A. Petersson, H. Nakatsuji, M. Caricato, X. Li, H. P. Hratchian, A. F. Izmaylov, J. Bloino, G. Zheng, J. L. Sonnenberg, M. Hada, M. Ehara, K. Toyota, R. Fukuda, J. Hasegawa, M. Ishida, T. Nakajima, Y. Honda, O. Kitao, H. Nakai, T. Vreven, J. A. Montgomery, Jr., J. E. Peralta, F. Ogliaro, M. Bearpark, J. J. Heyd, E. Brothers, K. N. Kudin, V. N. Staroverov, R. Kobayashi, J. Normand, K. Raghavachari, A. Rendell, J. C. Burant, S. S. Iyengar, J. Tomasi, M. Cossi, N. Rega, J. M. Millam, M. Klene, J. E. Knox, J. B. Cross, V. Bakken, C. Adamo, J. Jaramillo, R. Gomperts, R. E. Stratmann, O. Yazyev, A. J. Austin, R. Cammi, C. Pomelli, J. W. Ochterski, R. L. Martin, K. Morokuma, V. G. Zakrzewski, G. A. Voth, P. Salvador, J. J. Dannenberg, S. Dapprich, A. D. Daniels, O. Farkas, J. B. Foresman, J. V. Ortiz, J. Cioslowski, and D. J. Fox, , gaussian Inc. Wallingford CT 2009.

[5] P. Anger, P. Bharadwaj, and L. Novotny, Phys. Rev. Lett. **96**, 113002 (2006).

[6] K. Meguro, K. Sakamoto, R. Arafune, M. Satoh, and S. Ushioda, Phys. Rev. B **65**, 165405 (2002).
